# Supplementary material for: GPFL: A Gradient Projection-Based Client Selection Framework for Efficient Federated Learning
Source: arXiv:2403.17833 source file (2024-05-26)
Supplement: Supplementary file 1 [file 10Appendix.tex]

% \newpage
% \appendix




%Now, let's discuss the hyperparameters employed for each dataset and the different heterogeneous settings.
% \subsection{Model Construction and Hyperparameters}

% \subsubsection{Model Construction and Hyperparameters in FEMNIST}
% For the FEMNIST dataset, we adopt an MLP (Multi-Layer Perceptron) architecture with two hidden layers, consisting of 64 and 30  units, respectively.
% %following the methodology outlined in \cite{cho2022towards}. 
% In all three heterogeneous settings, the local batch size is set to 64, and the number of local iterations is set to 20. We initialize the learning rate ($\eta$) as 0.005. We utilize an SGD (Stochastic Gradient Descent) optimizer with a weight decay of 0.0001 and momentum of 0.1. The data is divided among $N = 100$ clients, with a participation fraction ($K$) of 10 for the 1SPC setting and 5 for the 2SPC and Dir settings.

% \subsubsection{Model Construction and Hyperparameters in CIFAR-10}
% For the CIFAR-10 dataset, we employ a CNN (Convolutional Neural Network) architecture with three convolutional layers, consisting of 32, 64, and 64 kernels, respectively, followed by a fully-connected layer with 64 units. In all three heterogeneous settings, the local batch size is set to 50, and the number of local iterations is set to 40. We use a fixed learning rate ($\eta$) of 0.01 without any learning rate decay and a weight decay of 0.0003 for the SGD optimizer. The total number of clients and the client participation fraction are consistent with those used in the FEMNIST dataset.

% By leveraging these specific hyperparameters and employing the respective neural models, we conducted federated learning experiments on the FEMNIST and CIFAR-10 datasets under different heterogeneous settings.


% % \Miya{This table is related to our experiment? If yes, put into appendix}
% % \begin{table*}[h]
% % \centering
% % \caption{Experimental parameters for evaluating a federated learning method.}
% % \label{tab:federated_learning_experiment_params}
% % \begin{tabular}{|c|c|c|c|c|c|c|c|}
% % \hline
% % \textbf{Experiment} & \textbf{Dataset} & \textbf{Total Clients} & \textbf{Selected Clients} & \textbf{Model} & \textbf{Learning Rate} & \textbf{Batch Size} \\ \hline
% % I & FEMNIST-tiny & 200 & 10 & CNN & 0.01 & 10 \\ \hline
% % II & FEMNIST & 3400 & 10 & CNN & 0.1 & 16 \\ \hline
% % III & FEMNIST & 3400 & 5 & CNN & 0.1 & 16  \\ \hline
% % IV & FedCIFAR100 & 500 & 10 & ResNet & 0.1 & 16 \\ \hline
% % V & CIFAR10 & 200 & 10 & CNN & 0.01 & 10 \\ \hline
% % \end{tabular}
% % \end{table*}
